# Supplementary material for: Distillation-guided Representation Learning for Unconstrained Gait Recognition
Source: arXiv:2307.14578 source file (2024-10-13)
Supplement: Supplementary file 1 [file supp.tex]

\setcounter{equation}{7}
\setcounter{table}{0}
\setcounter{figure}{0}

We provide additional
details on key sections as described below:
\begin{enumerate}
    \item \textbf{Gait Detector}: The visualizations of DHS patterns~(\ref{sec:visualization}), the architecture of gait detector~(\ref{sec:architecture}) the impact of gait detector~(\ref{sec:impact}) and failure cases~(\ref{sec:detectfail}).
    \item \textbf{Ratio and View-angle Correspondence}: ~(\ref{correspondence}).
    \item  \textbf{Experimental Details}: BRIAR dataset~(\ref{briar}), BRIAR visualizations~(\ref{briarvis}), implementation details~(\ref{Implementation}), CASIA-B evaluation~(\ref{casia-b}) and ablation study~(\ref{ablation})

\end{enumerate}

\section{Gait Detector}
\subsection{Visualization}
\label{sec:visualization}

\begin{figure*}[htb]
    \setlength{\abovecaptionskip}{2pt}
    \setlength{\tabcolsep}{2pt}
    \centering
    \begin{tabular}[b]{cccc}
        \begin{subfigure}[b]{.24\linewidth}
            \includegraphics[width= \textwidth,height=0.25\textwidth]{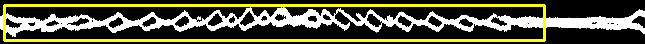}

        \end{subfigure} &
        \begin{subfigure}[b]{.24\linewidth}
            \includegraphics[width= \textwidth,height=0.25\textwidth]{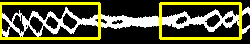}
        \end{subfigure}
        \begin{subfigure}[b]{.24\linewidth}
            \includegraphics[width= \textwidth,height=0.25\textwidth]{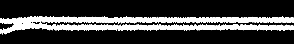}

        \end{subfigure} &
        \begin{subfigure}[b]{.24\linewidth}
            \includegraphics[width= \textwidth,height=0.25\textwidth]{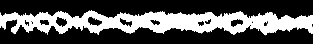}
        \end{subfigure} \\
        \begin{subfigure}[b]{.24\linewidth}
            \includegraphics[width= \textwidth,height=0.25\textwidth]{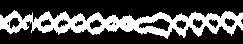}
        \end{subfigure} &
        \begin{subfigure}[b]{.24\linewidth}
            \includegraphics[width= \textwidth,height=0.25\textwidth]{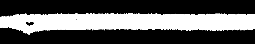}
        \end{subfigure}
        \begin{subfigure}[b]{.24\linewidth}
            \includegraphics[width= \textwidth,height=0.25\textwidth]{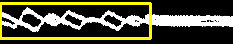}

        \end{subfigure} &
        \begin{subfigure}[b]{.24\linewidth}
            \includegraphics[width= \textwidth,height=0.25\textwidth]{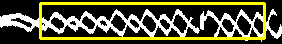} 
            \end{subfigure}\\
        \begin{subfigure}[b]{.24\linewidth}
            \includegraphics[width= \textwidth,height=0.25\textwidth]{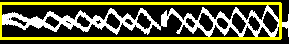}
        \end{subfigure} &
        \begin{subfigure}[b]{.24\linewidth}
            \includegraphics[width= \textwidth,height=0.25\textwidth]{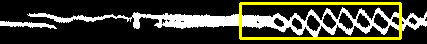}
        \end{subfigure}
        \begin{subfigure}[b]{.24\linewidth}
            \includegraphics[width= \textwidth,height=0.25\textwidth]{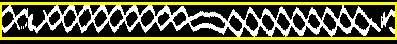}

        \end{subfigure} &
        \begin{subfigure}[b]{.24\linewidth}
            \includegraphics[width= \textwidth,height=0.25\textwidth]{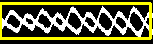} 
            \end{subfigure}\\
        \begin{subfigure}[b]{.24\linewidth}
            \includegraphics[width= \textwidth,height=0.25\textwidth]{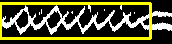}
        \end{subfigure} &
        \begin{subfigure}[b]{.24\linewidth}
            \includegraphics[width= \textwidth,height=0.25\textwidth]{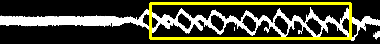}
        \end{subfigure}
        \begin{subfigure}[b]{.24\linewidth}
            \includegraphics[width= \textwidth,height=0.25\textwidth]{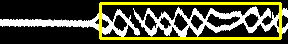}

        \end{subfigure} &
        \begin{subfigure}[b]{.24\linewidth}
            \includegraphics[width= \textwidth,height=0.25\textwidth]{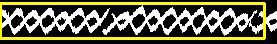} 
            \end{subfigure}\\
            \begin{subfigure}[b]{.24\linewidth}
            \includegraphics[width= \textwidth,height=0.25\textwidth]{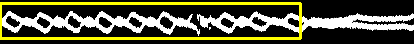}
        \end{subfigure} &
        \begin{subfigure}[b]{.24\linewidth}
            \includegraphics[width= \textwidth,height=0.25\textwidth]{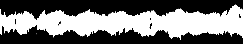}
        \end{subfigure}
        \begin{subfigure}[b]{.24\linewidth}
            \includegraphics[width= \textwidth,height=0.25\textwidth]{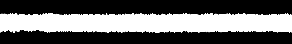}

        \end{subfigure} &
        \begin{subfigure}[b]{.24\linewidth}
            \includegraphics[width= \textwidth,height=0.25\textwidth]{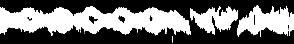} 
            \end{subfigure}\\
                \begin{subfigure}[b]{.24\linewidth}
            \includegraphics[width= \textwidth,height=0.25\textwidth]{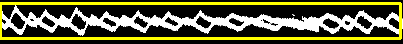}
        \end{subfigure} &
        \begin{subfigure}[b]{.24\linewidth}
            \includegraphics[width= \textwidth,height=0.25\textwidth]{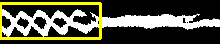}
        \end{subfigure}
        \begin{subfigure}[b]{.24\linewidth}
            \includegraphics[width= \textwidth,height=0.25\textwidth]{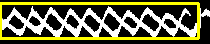}

        \end{subfigure} &
        \begin{subfigure}[b]{.24\linewidth}
            \includegraphics[width= \textwidth,height=0.25\textwidth]{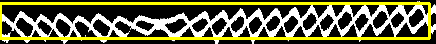} 
            \end{subfigure}\\
            \begin{subfigure}[b]{.24\linewidth}
            \includegraphics[width= \textwidth,height=0.25\textwidth]{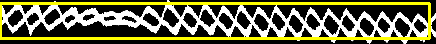}
        \end{subfigure} &
        \begin{subfigure}[b]{.24\linewidth}
            \includegraphics[width= \textwidth,height=0.25\textwidth]{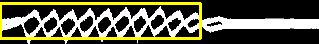}
        \end{subfigure}
        \begin{subfigure}[b]{.24\linewidth}
            \includegraphics[width= \textwidth,height=0.25\textwidth]{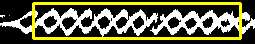}

        \end{subfigure} &
        \begin{subfigure}[b]{.24\linewidth}
            \includegraphics[width= \textwidth,height=0.25\textwidth]{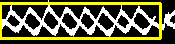} 
            \end{subfigure}\\
            \begin{subfigure}[b]{.24\linewidth}
            \includegraphics[width= \textwidth,height=0.25\textwidth]{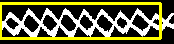}
        \end{subfigure} &
        \begin{subfigure}[b]{.24\linewidth}
            \includegraphics[width= \textwidth,height=0.25\textwidth]{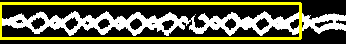}
        \end{subfigure}
        \begin{subfigure}[b]{.24\linewidth}
            \includegraphics[width= \textwidth,height=0.25\textwidth]{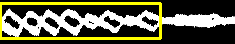}

        \end{subfigure} &
        \begin{subfigure}[b]{.24\linewidth}
            \includegraphics[width= \textwidth,height=0.25\textwidth]{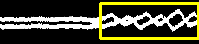} 
            \end{subfigure}\\
    \end{tabular}
    \caption{Visualization of DHS pattern and detector results on BRIAR.}
   \label{fig:DHS vis}
\vspace{-.2cm}
\end{figure*}

\begin{figure*}[!htb]
\vspace{-.2cm}
    \setlength{\abovecaptionskip}{1pt}
    \setlength{\tabcolsep}{2pt}
    \centering
    \begin{tabular}[b]{ccccc}
        \begin{subfigure}[b]{.19\linewidth}
            \includegraphics[width= \textwidth,height=0.25\textwidth]{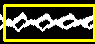}

        \end{subfigure} &
        \begin{subfigure}[b]{.19\linewidth}
            \includegraphics[width= \textwidth,height=0.25\textwidth]{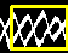}
        \end{subfigure}
        \begin{subfigure}[b]{.19\linewidth}
            \includegraphics[width= \textwidth,height=0.25\textwidth]{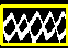}

        \end{subfigure} &
        \begin{subfigure}[b]{.19\linewidth}
            \includegraphics[width= \textwidth,height=0.25\textwidth]{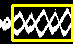}
        \end{subfigure}&
        \begin{subfigure}[b]{.19\linewidth}
            \includegraphics[width= \textwidth,height=0.25\textwidth]{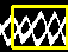}
        \end{subfigure} \\
        \begin{subfigure}[b]{.19\linewidth}
            \includegraphics[width= \textwidth,height=0.25\textwidth]{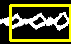}
        \end{subfigure} &
        \begin{subfigure}[b]{.19\linewidth}
            \includegraphics[width= \textwidth,height=0.25\textwidth]{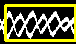}
        \end{subfigure}
        \begin{subfigure}[b]{.19\linewidth}
            \includegraphics[width= \textwidth,height=0.25\textwidth]{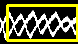}

        \end{subfigure} &
        \begin{subfigure}[b]{.19\linewidth}
            \includegraphics[width= \textwidth,height=0.25\textwidth]{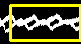} 
            \end{subfigure}&
        \begin{subfigure}[b]{.19\linewidth}
            \includegraphics[width= \textwidth,height=0.25\textwidth]{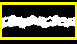}
        \end{subfigure} \\
    \end{tabular}
    \caption{Detector results on CASIA-B.}
   \label{fig:CASIA vis}
\end{figure*}

We provide some DHS patterns and gait detection results shown in \cref{fig:DHS vis}. The yellow box shows the detected gait sequence. We see that the gait detector accurately detects the gait appearance even in part of a sequence. Besides, there are visualizations on CAISA-B in \cref{fig:CASIA vis}. Our proposed gait detector can be smoothly exploited in CASIA-B dataset, even for extreme angles like 180\degree.

\subsection{Architecture}
\label{sec:architecture}
The detailed structure is shown in~\Cref{tab:strcture}. The input size is $L\times W$, where $L$ is equal to the length of the selected window, and the output of the model is a vector of size 4, representing the four classes. Only the full-gait sequences are used in our gait recognition model.

\begin{table}[h]

\centering
\begin{tabular}{  c c }
\hline
Module & Output Size \\

\hline
Input & 1$\times$ L $\times$ W\\
\hline
Conv1 \& maxpool &  16 $\times$  L $\times$ $\frac{1}{2}$W\\
\hline

Conv2 &  32 $\times$  L $\times$ $\frac{1}{2}$W\\
\hline
Conv3 \& maxpool &  32 $\times$  L $\times$ $\frac{1}{4}$W\\
\hline
Conv4 &  64 $\times$  L $\times$ $\frac{1}{4}$W\\
\hline
Conv5 &  64 $\times$  L $\times$ $\frac{1}{4}$W\\
\hline
Temporal Pool &  64$\times$  $\frac{1}{4}$W\\
\hline
MLP &  512\\
\hline
MLP &  4\\
\hline

\end{tabular}
\caption{Light-weighted classification structure in gait detector.}
\label{tab:strcture}
\end{table}

\subsection{Impact on Recognition Models}
\label{sec:impact}

Since the BRIAR dataset is an outdoor human authentication dataset with minimal curation, it provides an opportunity to evaluate both gait recognition and person identification (ReID). Specifically, we assess these models on sequences containing gait and static videos, respectively. We have observed that gait recognition tends to excel (42.5\% vs 28.4\%) on sequences containing gait but lags behind (7.8\% vs 28.9\%)\cite{lin2021gait, huang2023selfsupervised} person ReID methods on static videos. This disparity suggests that gait recognition places a stronger emphasis on temporal information compared to ReID. Consequently, we come up with a strategic approach wherein gait recognition serves as a filter, selectively directing qualified gait sequences for gait recognition, while the remaining sequences are processed by ReID. Through a complementary integration of the two models facilitated by a gait detector as an indicator, the overall performance reaches 37.8\%. This is in contrast to the individual performances of 28.3\% for gait recognition and 28.6\% for ReID when applied separately, highlighting the necessity of the gait detector in cooperation with gait recognition and ReID for achieving superior performance. 

In \Cref{tab:impact on ReID}, we employ a gait detector to assess the models' performance on classified sets. Specifically, the qualified set comprises the sequences involving gait with complete body, while the remaining are labeled as unqualified. ReID models exhibit a constant performance regardless of whether temporal information is included in the sequences. Conversely, gait recognition models display sensitivity to this fact, revealing a substantial over 20\% performance gap between the qualified and unqualified set. This underscores the efficacy of gait recognition in leveraging temporal information, while ReID excels on static videos. To capitalize this insight, we further conduct experiments on allocating qualified sequences to gait recognition and the rest to ReID. Consequently, we achieve SoTA performance on the BRIAR dataset.

\subsection{Failure Cases}
\label{sec:detectfail}

\noindent\textbf{Unqualified gait fragments appear even in curated dataset.}
We recognize the presence of unqualified gait fragments, such as incomplete body segments or sequences without discernible movement in the BRIAR dataset, simulating real-life gait recognition challenges. Previously, the quality of gait data received limited attention in prior methods, as most of datasets are curated. But with closer examination, we found this issue still exists. We show some examples from GREW~\cite{zhu2021gait} and Gait3D~\cite{zheng2022gait} in \cref{fig:curated}. We observe an incomplete body will cause body shape with large appearance differences due to normalization. These examples emphasize the importance of the gait detector even for curated datasets

\input{pictures/curatedfail}

\noindent\textbf{Analysis}
During test time, a fixed window length is used, which can result in \textit{missing} gait sequences or non-gait segments involved, as demonstrated in~\cref{fig:fail} first row, but the majority of the qualified sequence is still caught. Furthermore, since we only have accurate annotations for entire DHS sequences rather than individual moments, it is challenging to train a robust model to make correct predictions when the appearance is too similar, as shown in~\cref{fig:fail} second row. Despite these challenges, our gait detector is able to accurately identify the sequence qualification by employing 
gait proportion as a criterion in most cases, resulting in a significant improvement in the overall gait recognition performance.

\input{pictures/failure}

\section{Ratio and View-angle Correspondence}
\label{correspondence}
In the main paper Section 3.2.1, we demonstrate that there exists a correlation between the ratio
, which denotes the change in size from the original segmentation mask to the normalized body bounding box, and the viewpoint where the sequence is recorded. Thus, we embed the ratio into the model to implicitly utilize viewpoint information, resulting in improved performance. To verify this observation, we illustrate this relationship in Figure~\ref{fig:ratio}. In (a-e), we record the ratio change for each sequence at specific viewpoints. To have a better visualization, we place all the sequences at the same midpoint. Since the ratios for the same viewpoint follow a similar pattern, it is easy to distinguish the viewpoint using the ratio. In Figure~\ref{average}, we average the ratios for sequences recorded at the same angle and obtain a curve for each viewpoint. Ratio change is distinguishable, and we even observe symmetrical patterns at symmetric viewpoints, which propels us to incorporate ratio information into our gait recognition model as a cue for viewpoint information.

\begin{figure*}[htb]
    \setlength{\abovecaptionskip}{3pt}
    \setlength{\tabcolsep}{2pt}
    \centering
    \begin{tabular}[b]{ccc}
        \begin{subfigure}[b]{.33\linewidth}
            \includegraphics[clip, trim=0.0cm 0.25cm 0.0cm 1cm, width=1\textwidth,height=0.66\textwidth]{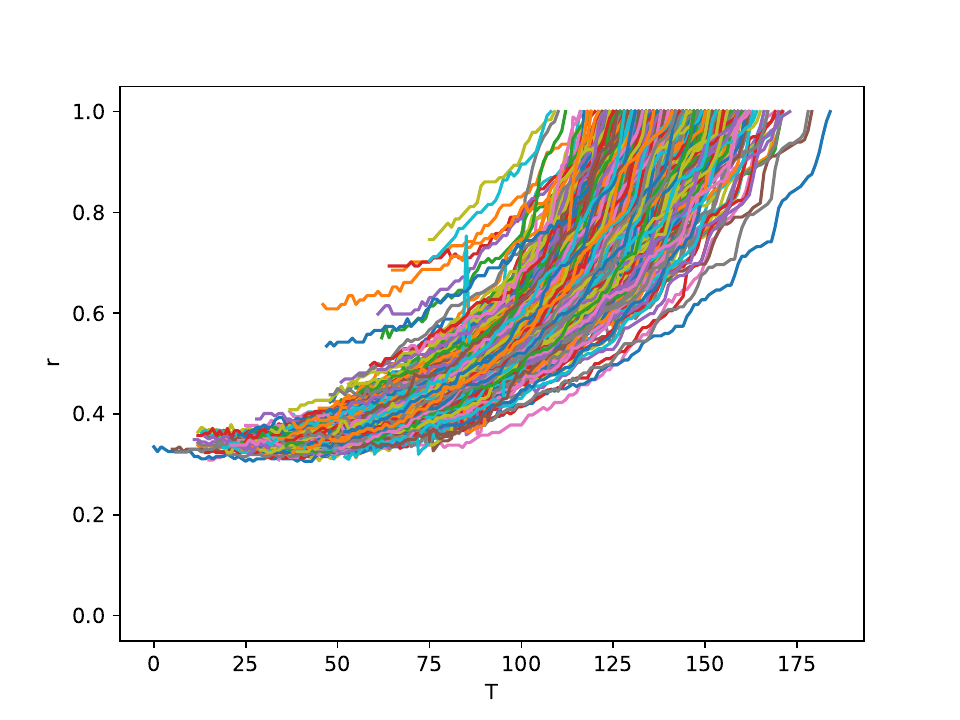}
            \caption{0 \degree}
            \label{0}
        \end{subfigure} &
        \begin{subfigure}[b]{.33\linewidth}
            \includegraphics[clip, trim=0.0cm 0.25cm 0.0cm 1cm,width=1\textwidth,height=0.66\textwidth]{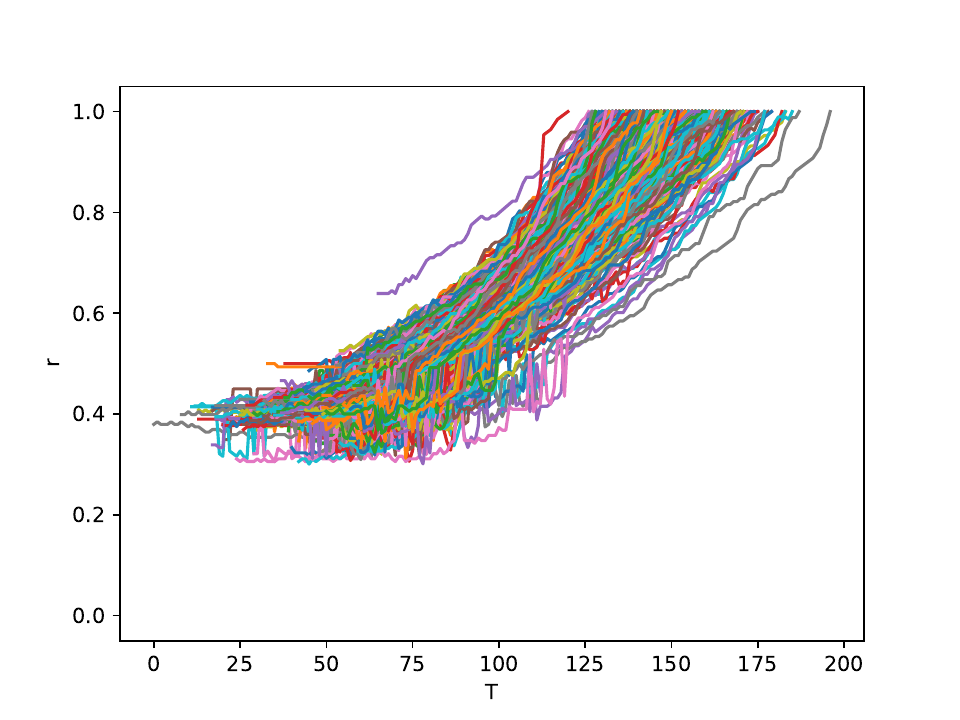}
            \caption{36 \degree}
            \label{36}
        \end{subfigure}&
        \begin{subfigure}[b]{.33\linewidth}
            \includegraphics[clip, trim=0.0cm 0.25cm 0.0cm 1cm,width=1\textwidth,height=0.66\textwidth]{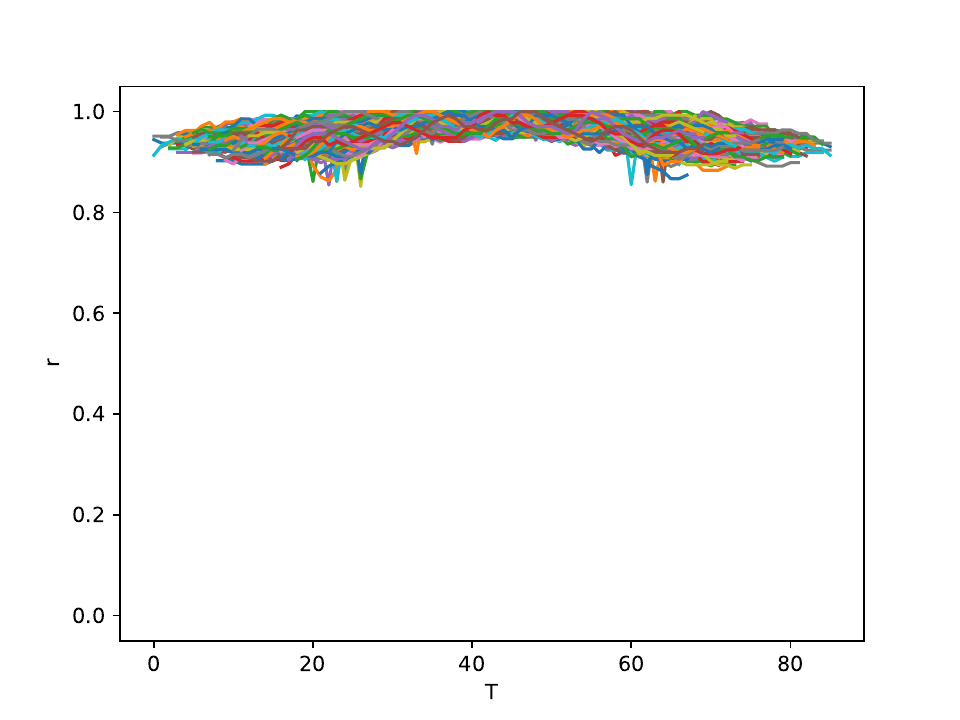}
            \caption{90 \degree}
            \label{90}
        \end{subfigure} \\[-1.25ex]%
        \begin{subfigure}[b]{.33\linewidth}
            \includegraphics[clip, trim=0.0cm 0.25cm 0.0cm 1cm,width=1\textwidth,height=0.66\textwidth]{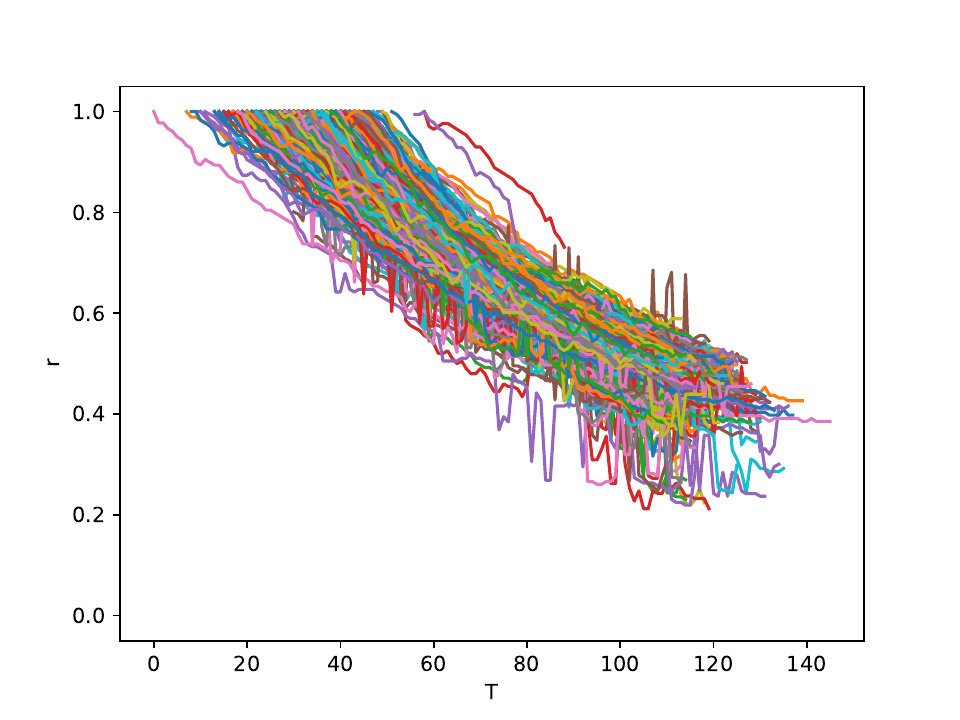}
            \caption{126 \degree}
            \label{126}
        \end{subfigure} &
        \begin{subfigure}[b]{.33\linewidth}
            \includegraphics[clip, trim=0.0cm 0.25cm 0.0cm 1cm,width=1\textwidth,height=0.66\textwidth]{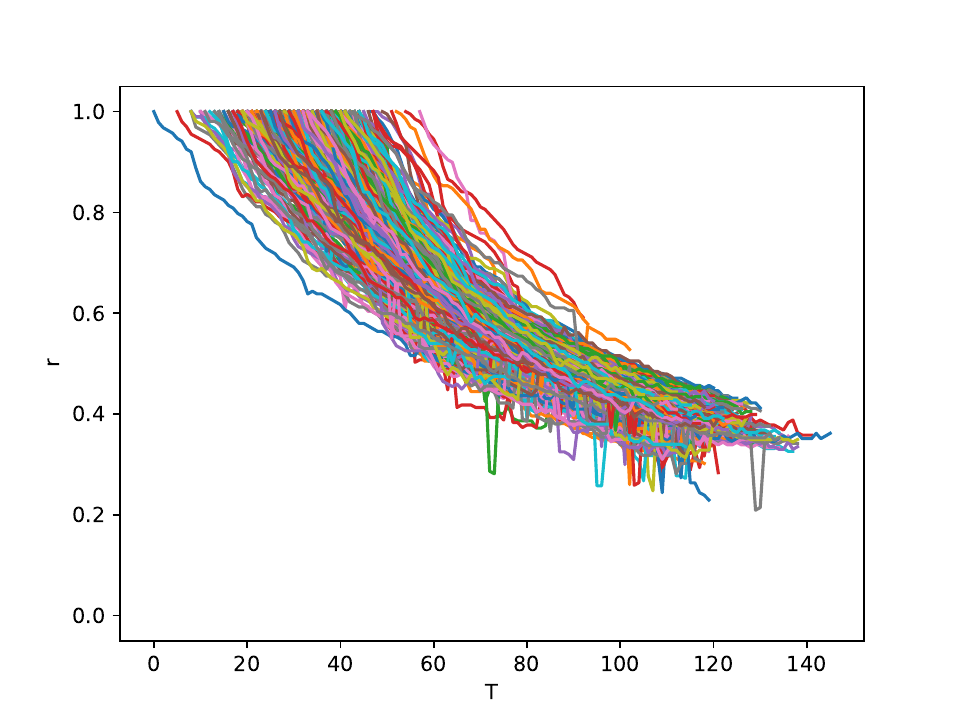}
            \caption{180 \degree}
            \label{180}
        \end{subfigure} &
        \begin{subfigure}[b]{.33\linewidth}
            \includegraphics[clip, trim=0.0cm 0.25cm 0.0cm 1cm,width=1\textwidth,height=0.66\textwidth]{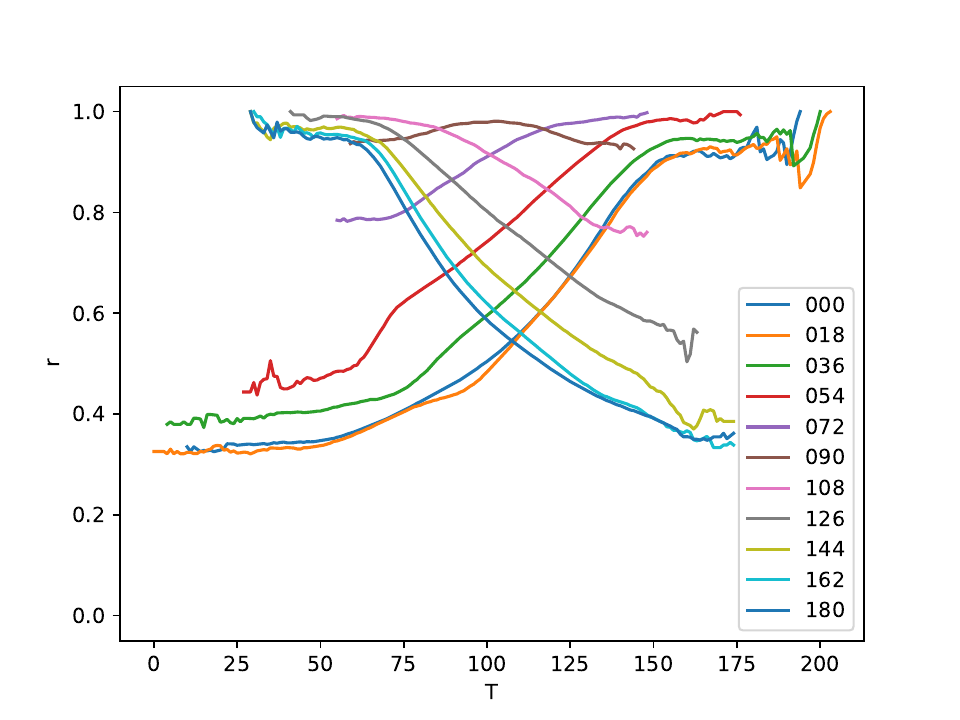}
            \caption{Average}
            \label{average}
        \end{subfigure} 
    \end{tabular}
\caption{The relationship between ratio and angles (a-e). And (f) shows the difference in average ratios at each angle. Each line represents the ratio change with time, and we centralize all lines to the same point to have a better visualization.}
   \label{fig:ratio}
\end{figure*}

\begin{table}
    \centering
    \begin{tabular}{cccc}
    \toprule
        Models & Qualified & Unqualified & Overall\\
        \midrule
        GaitSet & 30.4 & 8.3 & 17.6\\
        \rowcolor{GAR}$\hookrightarrow$w / GAR & 39.2 & 7.7 & 26.8 \\
        GaitPart & 28.1 & 8.2 & 15.7\\
        \rowcolor{GAR}$\hookrightarrow$w / GAR & 40.0 & 7.7 & 27.3 \\
        GaitGL & 29.8 & 6.7 & 17.3 \\
        \rowcolor{GAR}$\hookrightarrow$w / GAR & 42.5 & 7.8 & 28.3 \\
        GaitBase & 21.8 & 5.0 & 11.6 \\
        \rowcolor{GAR}$\hookrightarrow$w / GAR & 40.8 & 5.2 & 26.8 \\
        \midrule
        SemReID~\cite{huang2023selfsupervised} & 28.4  & 28.9 & 28.6 \\
        CAL~\cite{Gu_2022_CVPR} & 18.3 & 16.7 & 17.6 \\
        \bottomrule
    \end{tabular}
    \caption{The performance of gait recognition and person ReID models on BRIAR dataset with integration of gait detector. The qualified set represents the detected sequences containing periodic movement with complete body, and the unqualified are the remaining. }
    \label{tab:impact on ReID}
\end{table}

\section{Experimental Details}
\subsection{BRIAR Dataset}
\label{briar}
As shown in \cref{fig:vis}, BRIAR consists of 776 and 856 subjects used as training and test sets, respectively. In the test set, there are 493 distractors and 363 target subjects. For each identity, there are both indoor (\textit{controlled}) and outdoor (\textit{field}) sequences. The \textit{controlled} set is collected with 10 cameras from different viewing angles to record structure and random walking. In the \textit{field} set, the sequences are collected at varying distances and altitudes, namely close range (CR), 100m, 200m, 300m, 400m, 500m, 600m and unmanned aerial vehicle (UAV). There are also videos consisting of subjects standing all the time in the field set, as shown in \cref{fig:vis}. For each subject, two garment settings are applied, i.e. set1 and set2, to avoid clothing-based cues. The duration of each video is approximately 90 seconds. Human silhouettes are obtained using Detectron2~\cite{wu2019detectron2}.

\begin{figure}[!tb]
    \setlength{\abovecaptionskip}{3pt}
    \setlength{\tabcolsep}{0pt}
    
    \setlength{\belowcaptionskip}{-0.2cm}
    \centering
    \begin{tabular}[c]{cccccccc}
    
        \begin{subfigure}[b]{.12\linewidth}
             \includegraphics[width=\textwidth,height=1.5\textwidth]{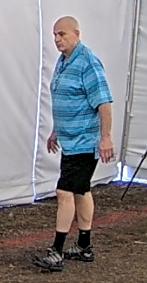}
                \label{fig:72controlled}
        \end{subfigure}&
        \begin{subfigure}[b]{.12\linewidth}
             \includegraphics[width=\textwidth,height=1.5\textwidth]{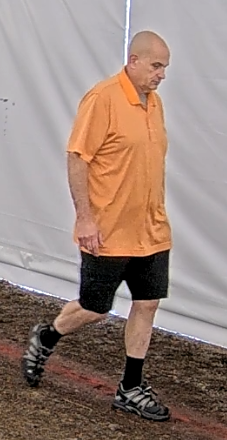}
                \label{fig:72}
        \end{subfigure}&
        \begin{subfigure}[b]{.12\linewidth}
             \includegraphics[width=\textwidth,height=1.5\textwidth]{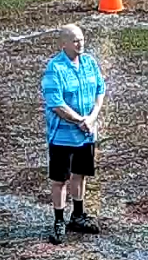}
                \label{fig:265_100_set2}
        \end{subfigure}&
        \begin{subfigure}[b]{.12\linewidth}
             \includegraphics[width=\textwidth,height=1.5\textwidth]{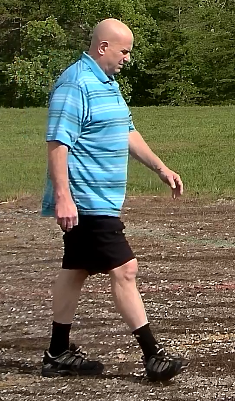}
                \label{fig:265_close}
        \end{subfigure}&
        \begin{subfigure}[b]{.12\linewidth}
             \includegraphics[width=\textwidth,height=1.5\textwidth]{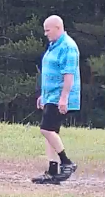}
                \label{fig:265_200}
        \end{subfigure}&
        \begin{subfigure}[b]{.12\linewidth}
             \includegraphics[width=\textwidth,height=1.5\textwidth]{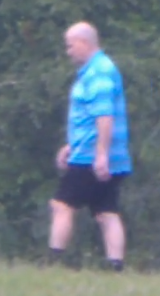}
                \label{fig:265_400}
        \end{subfigure}&
        \begin{subfigure}[b]{.12\linewidth}
             \includegraphics[width=\textwidth,height=1.5\textwidth]{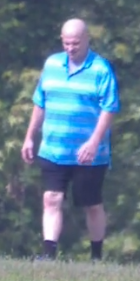}
                \label{fig:265_500}
        \end{subfigure}&
        \begin{subfigure}[b]{.12\linewidth}
             \includegraphics[width=\textwidth,height=1.5\textwidth]{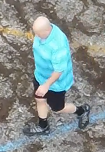}
                \label{fig:265_uav}
        \end{subfigure}
        \vspace{-1.2em} \\
        \begin{subfigure}[b]{.12\linewidth}
             \includegraphics[width=\textwidth,height=1.5\textwidth]{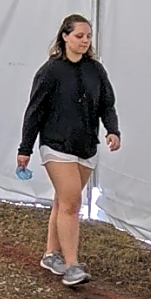}
                \label{fig:265controlled}
        \end{subfigure}&
        
        \begin{subfigure}[b]{.12\linewidth}
             \includegraphics[width=\textwidth,height=1.5\textwidth]{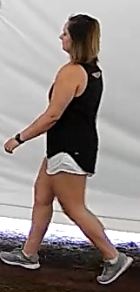}
                \label{fig:265_100}
        \end{subfigure}&
        \begin{subfigure}[b]{.12\linewidth}
             \includegraphics[width=\textwidth,height=1.5\textwidth]{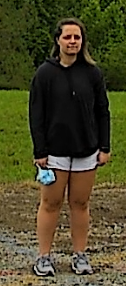}
                \label{fig:265_100_set2}
        \end{subfigure}&
        \begin{subfigure}[b]{.12\linewidth}
             \includegraphics[width=\textwidth,height=1.5\textwidth]{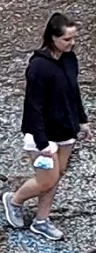}
                \label{fig:265_close}
        \end{subfigure}&
        \begin{subfigure}[b]{.12\linewidth}
             \includegraphics[width=\textwidth,height=1.5\textwidth]{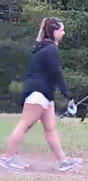}
                \label{fig:265_200}
        \end{subfigure}&
        \begin{subfigure}[b]{.12\linewidth}
             \includegraphics[width=\textwidth,height=1.5\textwidth]{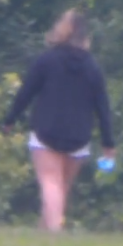}
                \label{fig:265_400}
        \end{subfigure}&
        \begin{subfigure}[b]{.12\linewidth}
             \includegraphics[width=\textwidth,height=1.5\textwidth]{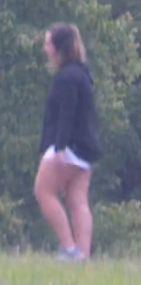}
                \label{fig:265_500}
        \end{subfigure}&
        \begin{subfigure}[b]{.12\linewidth}
             \includegraphics[width=\textwidth,height=1.5\textwidth]{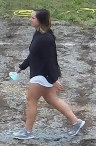}
                \label{fig:265_uav}
        \end{subfigure}
        \vspace{-1.2em} \\
        \begin{subfigure}[b]{.12\linewidth}
             \includegraphics[width=\textwidth,height=1.5\textwidth]{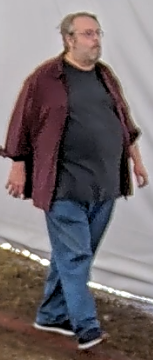}
                \label{fig:265controlled}
        \end{subfigure}&
        
        \begin{subfigure}[b]{.12\linewidth}
             \includegraphics[width=\textwidth,height=1.5\textwidth]{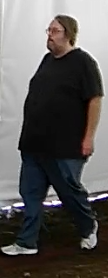}
                \label{fig:265_100}
        \end{subfigure}&
        \begin{subfigure}[b]{.12\linewidth}
             \includegraphics[width=\textwidth,height=1.5\textwidth]{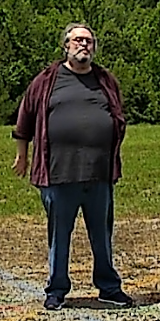}
                \label{fig:265_100_set2}
        \end{subfigure}&
        \begin{subfigure}[b]{.12\linewidth}
             \includegraphics[width=\textwidth,height=1.5\textwidth]{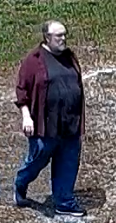}
                \label{fig:265_close}
        \end{subfigure}&
        \begin{subfigure}[b]{.12\linewidth}
             \includegraphics[width=\textwidth,height=1.5\textwidth]{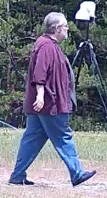}
                \label{fig:265_200}
        \end{subfigure}&
        \begin{subfigure}[b]{.12\linewidth}
             \includegraphics[width=\textwidth,height=1.5\textwidth]{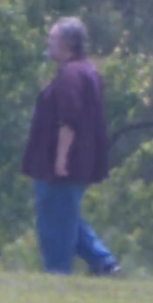}
                \label{fig:265_400}
        \end{subfigure}&
        \begin{subfigure}[b]{.12\linewidth}
             \includegraphics[width=\textwidth,height=1.5\textwidth]{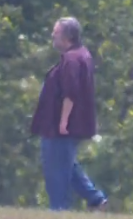}
                \label{fig:265_500}
        \end{subfigure}&
        \begin{subfigure}[b]{.12\linewidth}
             \includegraphics[width=\textwidth,height=1.5\textwidth]{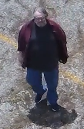}
                \label{fig:265_uav}
        \end{subfigure}
        \vspace{-1.2em} \\
        \begin{subfigure}[b]{.12\linewidth}
             \includegraphics[width=\textwidth,height=1.5\textwidth]{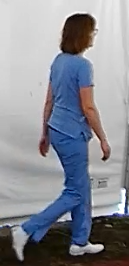}
                \label{fig:265controlled}
        \end{subfigure}&
        
        \begin{subfigure}[b]{.12\linewidth}
             \includegraphics[width=\textwidth,height=1.5\textwidth]{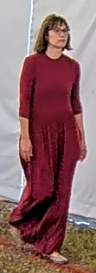}
                \label{fig:265_100}
        \end{subfigure}&
        \begin{subfigure}[b]{.12\linewidth}
             \includegraphics[width=\textwidth,height=1.5\textwidth]{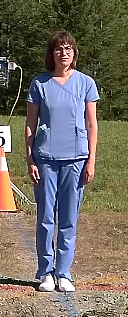}
                \label{fig:265_100_set2}
        \end{subfigure}&
        \begin{subfigure}[b]{.12\linewidth}
             \includegraphics[width=\textwidth,height=1.5\textwidth]{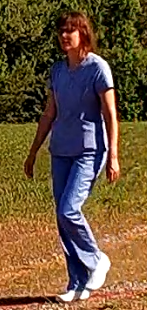}
                \label{fig:265_close}
        \end{subfigure}&
        \begin{subfigure}[b]{.12\linewidth}
             \includegraphics[width=\textwidth,height=1.5\textwidth]{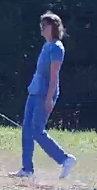}
                \label{fig:265_200}
        \end{subfigure}&
        \begin{subfigure}[b]{.12\linewidth}
             \includegraphics[width=\textwidth,height=1.5\textwidth]{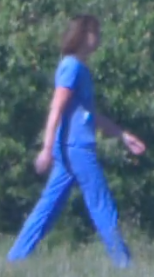}
                \label{fig:265_400}
        \end{subfigure}&
        \begin{subfigure}[b]{.12\linewidth}
             \includegraphics[width=\textwidth,height=1.5\textwidth]{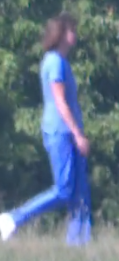}
                \label{fig:265_500}
        \end{subfigure}&
        \begin{subfigure}[b]{.12\linewidth}
             \includegraphics[width=\textwidth,height=1.5\textwidth]{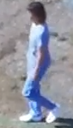}
                \label{fig:265_uav}
        \end{subfigure}
        \vspace{-1.2em} \\
        \begin{subfigure}[b]{.12\linewidth}
             \includegraphics[width=\textwidth,height=1.5\textwidth]{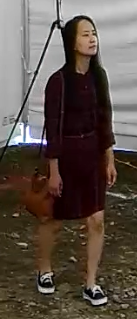}
                \label{fig:265controlled}
        \end{subfigure}&
        
        \begin{subfigure}[b]{.12\linewidth}
             \includegraphics[width=\textwidth,height=1.5\textwidth]{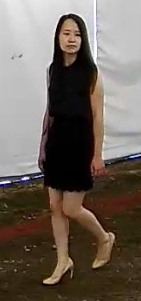}
                \label{fig:265_100}
        \end{subfigure}&
        \begin{subfigure}[b]{.12\linewidth}
             \includegraphics[width=\textwidth,height=1.5\textwidth]{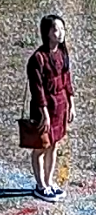}
                \label{fig:265_100_set2}
        \end{subfigure}&
        \begin{subfigure}[b]{.12\linewidth}
             \includegraphics[width=\textwidth,height=1.5\textwidth]{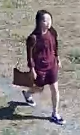}
                \label{fig:265_close}
        \end{subfigure}&
        \begin{subfigure}[b]{.12\linewidth}
             \includegraphics[width=\textwidth,height=1.5\textwidth]{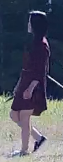}
                \label{fig:265_200}
        \end{subfigure}&
        \begin{subfigure}[b]{.12\linewidth}
             \includegraphics[width=\textwidth,height=1.5\textwidth]{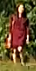}
                \label{fig:265_400}
        \end{subfigure}&
        \begin{subfigure}[b]{.12\linewidth}
             \includegraphics[width=\textwidth,height=1.5\textwidth]{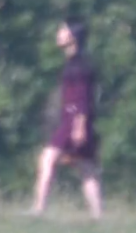}
                \label{fig:265_500}
        \end{subfigure}&
        \begin{subfigure}[b]{.12\linewidth}
             \includegraphics[width=\textwidth,height=1.5\textwidth]{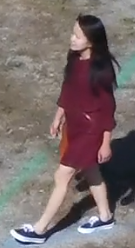}
                \label{fig:265_uav}
        \end{subfigure}
        \vspace{-1.2em} \\
        
    \end{tabular}
    \caption{Examples of subjects in different conditions from the BRIAR dataset at different distances attitudes and clothing. The columns represent controlled-set1, controlled-set2, CR-stand, CR-walk, 100m, 400m, 500m and UAV respectively. Sample videos are in the \textbf{supplementary material} section. All the subjects shown have consented to the publication of their images.}
    \vspace{-4mm}
    \label{fig:vis}
\end{figure}

\subsection{BRIAR Visualization}
\label{briarvis}
Compared to most widely used constrained datasets, like CASIA-B~\cite{yu2006framework} and OU-MVLP~\cite{takemura2018multi}, BRIAR~\cite{briar} is a more challenging one, due to its instability. It contains outdoor sequences with variations in appearance change, such as clothing settings, atmospheric turbulence, altitudes (ground, elevated level and in the air), and walking settings, i.e. random walking and structure walking and non-walking sequence (standing). And even in walking sequences, there are clips containing standing. These scenes mimic real-world gait patterns. To have an intuitive feel about the dataset, we show some example clips in the folder namely \url{./clips/}. In the folder, we show the video recorded in \textbf{different platforms}, i.e.\url{ controlled_rand.mp4}, \url{ 100m_set1.mp4} and \url{ uav.mp4}, \textbf{various distances}, i.e.\url{ close_high.mp4}, \url{ 100m_set1.mp4}, \url{ 400m.mp4}, and \url{ 500m.mp4}, \textbf{different altitudes}, i.e. \url{ close_high.mp4}, \url{ uav.mp4} and \url{ 100m_set1.mp4}, \textbf{clothes changing}, i.e. \url{ 100m_set1.mp4} and \url{ 100m_set2_stand.mp4} and \textbf{diverse movement types}, i.e. \url{ 100m_set2_stand.mp4} \url{ controlled_struct.mp4} and \url{ controlled_rand.mp4}. 
And it is noticeable that \url{ 100m_set2.mp4} is an example of an incomplete body due to vegetation occlusion, and our gait detector can filter it out. All the subjects shown have consented to the publication of their images.

\subsection{Implementation Details}
\label{Implementation}
All experiments are implemented in Pytorch~\cite{paszke2019pytorch} with four NVIDIA A5000 GPUs. We follow~\cite{chao2019gaitset} to obtain normalized silhouettes and RGB body chips at the resolution of $64\times64$ from the original segmentation masks and frames for CASIA-B and BRIAR. The resizing ratio is also recorded during the normalization process. For CASIA-B, we follow the configurations of the widely used gait feature extraction models, i.e. GaitSet~\cite{chao2019gaitset}, GaitPart~\cite{fan2020gaitpart}, GaitGL~\cite{lin2021gait} and GaitBase~\cite{fan2023opengait}, to extract RGB and silhouette feature. 
For the BRIAR dataset, we use a larger version of these architectures designed for OU-MVLP~\cite{takemura2018multi}, considering the number of identities and scene complexity. And we implement the experiments using~\cite{fan2023opengait}. In the training phase, the batch size for both datasets is (8,8), i.e. eight subjects with eight videos per subject for each batch. Thirty continuous frames are randomly sampled from a video. %

Our gait detector is trained using DHS generated from the BRIAR training set in a supervised manner using annotations provided by the BRIAR program. To ensure robustness to varying time duration, we randomly select input lengths ranging from 30 to 100 for each iteration. The detector is evaluated on DHS from the testing sets of three datasets. Specifically, we select window sizes of 33, 50, and 80. The confidence and overlapping threshold are 0.9 and 0.3 for NMS. The performance is evaluated using average accuracy, where correctness means more than 50\% of the sequence has predictions matching with the ground truth. Considering CASIA-B and Gait3D are pure gait datasets, we suppose all sequences in these datasets as complete body gait. Therefore, we do not further evaluate GADER. For the BRIAR dataset, we use the proposed gait detector to filter the qualified sequences fed to the GAR model, and the rest of the sequences are processed by a SoTA ReID method, SemReID~\cite{huang2023selfsupervised}.

\subsection{CASIA-B Evaluation}
\label{casia-b}

We also provide complete evaluation on CASIA-B dataset, shown in ~\Cref{tab:CASIA-B_Rank}. 
Compared to the original backbones, the models with prior knowledge consistently demonstrate superior performance. There are enhancements of 0.7\%, 1.8\% and 3.3\% for GaitSet on NM, BG and CL respectively. Notably, while the original GaitBase already exhibits high performance in NM, it still gains a 0.6\% increase by collaborating with GAR, reaching 98.2\%. It shows that the proposed GAR can improve every backbones through prior knowledge from RGB and viewing angles.

\begin{table*}[!htb]
\small
\centering
\begin{tabular}{ c | c |c |c |c |c |c |c |c |c |c |c |c |l }
\hline
\multicolumn{2}{c|}{Gallery NM\#1-4} & \multicolumn{12}{c}{$0\degree - 180\degree$}\\
\hline
\multicolumn{2}{c|}{Probe} & $0\degree$ & $18\degree$ & $36\degree$ & $54\degree$ & $72\degree$& $90\degree$& $108\degree$ & $126\degree$ & $144\degree$& $162\degree$& $180\degree$& Mean \\

\hline
\multirow{9}{*}{NM\#1-2} 

 & GaitSet~\cite{chao2019gaitset} & 90.8 & 97.9 & 99.4 & 96.9 & 93.6 & 91.7 & 95.0 & 97.8 & 98.9 & 96.8 & 85.8 & 95.0 \\
 \rowcolor{GAR} \cellcolor[rgb]{1,1,1} &  $\hookrightarrow$ w / GAR & 91.7 & 98.3 & 99.1 & 97.7 & 94.9 & 93.1 & 94.9 & 97.6 & 98.8 & 98.0 & 88.9 & 95.7 \small \textcolor{green}{$\uparrow$ 0.7} \\

 & GaitPart~\cite{fan2020gaitpart} & 94.1 & 98.6 & 99.3 & 98.5 &  94.0 & 92.3 & 95.9 & 98.4 & 99.2 & 97.8 & 90.4 & 96.2\\ 
  \rowcolor{GAR} \cellcolor[rgb]{1,1,1} & $\hookrightarrow$ w / GAR & 93.6 & 98.3 & 99.5 & 99.5 & 94.9 & 92.8 & 95.2 & 98.3 & 98.9 & 97.6 & 89.7 & 96.3 \small \textcolor{green}{$\uparrow$ 0.1}\\

  & GaitBase~\cite{fan2023opengait}  & - &- & - & - & - & - & - & - & - & -& - & 97.6  \\
    \rowcolor{GAR} \cellcolor[rgb]{1,1,1} & $\hookrightarrow$ w / GAR & 95.1 & \textbf{99.8} & \textbf{99.9} & \textbf{99.7}& \textbf{97.8} & \textbf{97.5} & \textbf{97.9} & \textbf{99.6} & \textbf{99.8} & \textbf{99.3} & \textbf{94.1} & \textbf{98.2} \small \textcolor{green}{$\uparrow$ 0.6}\\
    
 & GaitGL~\cite{lin2021gait} & 96.0 & 98.3 & 99.0 & 97.9 & 96.9 & 95.4 & 97.0 & 98.9 & 99.3 & 98.8 & 94.0 & 97.4 \\  
  \rowcolor{GAR} \cellcolor[rgb]{1,1,1} &$\hookrightarrow$ w / GAR & \textbf{97.1} & 98.7 & 99.0 & 97.9 & 96.4 & 95.6 & 97.7 & 98.8 & 99.0 & 98.4 & \textbf{94.1} & 97.5 \small \textcolor{green}{$\uparrow$ 0.1}\\

\hline
\multirow{9}{*}{BG\#1-2}

 & GaitSet~\cite{chao2019gaitset} & 83.8 & 91.2 & 91.8 & 88.8 & 83.3 & 81.0 & 84.1 & 90.0 & 92.2 & 94.4 & 79.0 & 87.2 \\
 \rowcolor{GAR} \cellcolor[rgb]{1,1,1} &  $\hookrightarrow$ w / GAR & 87.8 & 92.9 & 93.1 & 91.6 &86.1 & 81.3 & 86.7 & 90.7 & 94.6 & 92.3 & 82.0 &89.0 \small \textcolor{green}{$\uparrow$ 1.8} \\

 & GaitPart~\cite{fan2020gaitpart} & 89.1 & 94.8 & 96.7 & 95.1 &  88.3 & 84.9 & 89.0 & 93.5 & 96.1 & 93.8 & 85.8 & 91.5\\ 
  \rowcolor{GAR} \cellcolor[rgb]{1,1,1} & $\hookrightarrow$ w / GAR & 90.7 & 95.1 & 97.1 & \textbf{96.4} & 88.7 & 81.1 & 87.5 & 95.3 & 97.9 & 96.9 & 87.5 & 92.2 \small \textcolor{green}{$\uparrow$ 0.7}\\

  & GaitBase~\cite{fan2023opengait}  & - &- & - & - & - & - & - & - & - & -& - & 94.0  \\
    \rowcolor{GAR} \cellcolor[rgb]{1,1,1} & $\hookrightarrow$ w / GAR & 92.7 & 96.4 & 96.2 & 96.0& 92.6 & 89.1 & 91.1 & 95.7 & 97.3 & 96.0 & 90.7& 94.0 --\\
    
 & GaitGL~\cite{lin2021gait} & 92.6 & \textbf{96.6} & 96.8 & 95.5 & 93.5 & 89.3 & \textbf{92.2} & \textbf{96.5} & 98.2 & 96.9 & 91.5 & 94.5 \\  
  \rowcolor{GAR} \cellcolor[rgb]{1,1,1} &$\hookrightarrow$ w / GAR & \textbf{92.9} & 95.9 & 96.5 & 95.2 & \textbf{94.5} & \textbf{89.5} & 92.0 & \textbf{96.5} & 98.0 & 96.9 & 91.7 & 94.5  \small --\\

\hline
\multirow{9}{*}{CL\#1-2} 

 & GaitSet~\cite{chao2019gaitset} & 61.4 & 75.4 & 80.7 & 77.3 & 72.1 & 70.1 & 71.5 & 73.5 & 73.5 & 68.4 & 50.0 & 70.4 \\
 \rowcolor{GAR} \cellcolor[rgb]{1,1,1} &  $\hookrightarrow$ w / GAR & 67.5 & 82.3 & 84.1 & 79.2 & 70.8 & 68.8 & 71.4 & 75.2 & 77.7 & 75.9 & 58.1 &73.7 \small \textcolor{green}{$\uparrow$ 3.3} \\

 & GaitPart~\cite{fan2020gaitpart} & 70.7 & 85.5 & 86.9 & 83.3 &  77.1 & 72.5 & 76.9 & 82.2 & 83.8 & 80.2 & 66.5 & 78.7\\ 
  \rowcolor{GAR} \cellcolor[rgb]{1,1,1} & $\hookrightarrow$ w / GAR & 78.0 & 85.7 & 89.4 & 84.4 & 77.7 & 71.6 & 77.0 & 79.7 & 84.3 & 81.3 & 68.2 & 79.7 \small \textcolor{green}{$\uparrow$ 1.0}\\

  & GaitBase~\cite{fan2023opengait}  & - &-   &- &- &- &- &- &- &- &- &- & 77.4  \\
    \rowcolor{GAR} \cellcolor[rgb]{1,1,1} & $\hookrightarrow$ w / GAR & 69.3 & 80.1 & 82.5 & 82.1& 81.2 & 78.2 & 77.8 & 80.0 & 83.3 & 80.2 & 65.3 & 78.2 \small \textcolor{green}{$\uparrow$ 0.8}\\
    
 & GaitGL~\cite{lin2021gait} & 76.6 & 90.0 & 90.3 & 87.1 & 84.5 & 79.0 & 84.1 & 87.0 & 87.3 & 84.4 & 69.5 & 83.6 \\  
  \rowcolor{GAR} \cellcolor[rgb]{1,1,1} &$\hookrightarrow$ w / GAR & 80.8 & \textbf{90.5} & \textbf{92.2} & 91.0 & 84.7 & \textbf{79.7} & \textbf{84.8} & 89.6 & 89.7 & \textbf{87.1} & \textbf{72.8} & 85.7  \small \textcolor{green}{$\uparrow$ 2.1}\\
 
\hline
\end{tabular}
\caption{Rank-1 accuracy (\%) on CASIA-B  excluding identical-view case for NM\#1-2, BG\#1-2 and CL\#1-2.}
\label{tab:CASIA-B_Rank}
\vspace{-4mm}
\end{table*}

\subsection{Ablation Study}
\label{ablation}
   \begin{table}[h]

\centering
\small
\begin{tabular}{  c |c|c |c| c }
\hline
Methods   & NM & BG & CL & Mean \\
\hline
None & 97.4 &94.5 &83.6 & 91.8 \\
\hline
Add & 95.9 & 92.1 &  81.5 &  89.8\\

 \cline{2-5}
Concat & 97.2 & 94.4 &  83.9 &  91.8\\

\hline
\textbf{Attention (Ours)} & 97.4 & 94.4 & 85.1 & 92.3\\

\hline

\end{tabular}
\caption{Rank-1 accuracy on CASIA-B using different ratio fusion methods.}
\label{tab:fusion}
\vspace{-3mm}
\end{table}

\noindent\textbf{Comparison with different fusion approaches for ratio.}
To seek a suitable method to incorporate the ratio information into the pipeline, we conducted a comprehensive set of experiments to compare various fusion strategies. Apart from attention, we also introduced two alternative operations: `Add' and `Concat'. The `Add' involves directly adding the ratio feature space to the frames' feature space, while the `Concat' is to concatenate them by expanding the ratio embedding to match the frames' feature size. All combinations are conducted at a consistent location, specifically, the features at the first 3D convolution layers within the RGB and silhouette feature extraction backbones. From Table~\ref{tab:fusion}, we find that our approach gains a mean accuracy improvement of +0.5\% over the concatenation-based method. So we apply attention to encode the ratio information.
